# Supplementary material for: Point-Based Value Iteration for POMDPs with Neural Perception Mechanisms
Source: arXiv:2306.17639 source file (2024-08-07)
Supplement: Supplementary file 1 [file appendix_case_studies.tex]

\section{Case Studies -- Further Details}\label{case-app}

In this section we give the complete descriptions of our two case studies as well as some additional analysis.
%\gethin{needs editing}
%The particle-based initial beliefs were generated as follows: select an agent state, sample a finite set of percept compatible environment states, and assign positive probabilities to these states, while the region-based initial beliefs were generated as follows: select an agent state, sample a finite set of regions of percept compatible environment states, and set the belief as the uniform distribution over each region. 
For both the car parking example and the VCAS, we use the method of  \cite{KM-FF:20} to compute the preimage of piecewise linear NNs which iterates backwards through the layers. %, building it layer by layer. %the preimage from the preimage of each layer. 
This method is %naturally 
only applicable when the NN has piecewise linear boundaries, for which the basic building blocks are polytopes which include NNs with ReLU or linear layers.  With this preimage, we then construct a polyhedral representation of the environment space corresponding to the perception FCP.
%according to how the points inside the regions for each iteration are classified or observed by the agent. \gethinM{new FCP - do you mean perception FCP (if not I do not follow what you mean by "will be classified"} 
%\ruiM{sorry, this is from the old one. Please check} \gethinM{do we need to say more than just perception FCP here?}\ruiM{i don't find other aspects to say at the moment}
Regarding boundary points, we order regions and then assign boundary points to the region with highest order, resolving ties via a measurable rule. We emphasize that, although the states in any region of the perception FCP are observationally equivalent, they can have different values because they lead to paths that are not observationally equivalent.

%\gethinM{what does highest order mean?} \ruiM{If a boundary point is shared by multiple regions which have different orders, then the class of this point is the same as the class of the region with the highest order. Essentially we are ordering the percepts} \gethinM{how are you ordering and why is it the right ordering?} \ruiM{From a theoretical view, we only need a measurable way to decide the classes of boundary points, and ordering the classes is a solution. From an implementation view, we only consider strict inequalities to represent a region, which means we never worry about breaking the tie. This is supported by the fact that the measure of boundary points is zero (we add a very small number to disturb the state if the boundary point is unfortunate to occur). Please check}
%, thus ensuring the Borel measurability required for the value function \cite{nscsgs}. \gethin{suggest remove this last part as not mentioned previously}

\subsection{Car Parking Case Study} 

This case study is the dynamic vehicle parking problem from \egref{ex:parking:model} which we extend with both with obstacles and to a larger environment. We first give the full details of the original NS-POMDP and then present the changes when obstacles are added and the larger environment is considered.

\startpara{$4 {\times} 4$ environment} As in \egref{ex:parking:model}, a vehicle is looking for a parking spot $\mathcal{R}_P = \{(x, y) \in \mathbb{R}^2 \mid 2 \leq x \leq 3 \wedge 3 \leq y \leq 4\}$ in a $4 {\times} 4$ continuous environment. Formally, it can be modeled as an NS-POMDP where:
\begin{itemize}
	\item $S_A= \Loc \times \Per$ where  $\Loc = \{1,\dots,5\}$ (local states) are the 5 trust levels and $\Per = \{ 1, \dots, 16 \}$ (percepts) are the 16 abstract grid points which are ordered according to \tabref{tab:advisory-parking};

	\item $S_E = \mathcal{R}= \{(x, y) \in \mathbb{R}^2 \mid 0 \leq x, y \leq 4\}$;
	
	\item $Act = \{ \mathit{up}, \mathit{down}, \mathit{left}, \mathit{right}, \mathit{parking} \}$;

	\item $\Delta_A(tr, \per) = \Act$ if $\per = 15$, and $\Delta_A(tr, \per) = \{ \mathit{up}, \mathit{down}, \mathit{left}, \mathit{right} \} $ otherwise for all $tr \in \Loc$ and $\per \in \Per$;

	 \item $\obs_A(tr,(x, y))=\argmax (f(x, y))$, where $f$ is implemented via a feed-forward NN with one ReLU hidden-layer and 14 neuros, takes the coordinate vector of the vehicle as input and then outputs one of the 16 abstract grid points (\figref{fig:car_parking}, middle). The boundary coordinate is resolved by assigning the grid point with the smallest label; 

    \item for $s_A=(tr, \per) \in S_A$, $tr' \in \Loc$ and $a \in \Act$, if $a$ is compliant with $\per$, see \tabref{tab:advisory-parking}, then:
     \[
     \delta_A(s_A,a)(\tr') = \left\{ \begin{array}{cl}
     1  & \mbox{if $(\tr\leq4) \wedge (\tr'=\tr+1)$} \\
     1 & \mbox{if $(\tr=5) \wedge (\tr'=\tr)$} \\
     0 & \mbox{otherwise}
     \end{array}  \right.
     \]
    on the other hand, if $a$ is not compliant with $\per$, then:
     \[
     \delta_A(s_A,a)(\tr') = \left\{ \begin{array}{cl}
     \lambda & \mbox{if $(\tr\geq 2) \wedge (\tr'=\tr-1) $} \\
     1-\lambda & \mbox{if $(\tr\geq 2) \wedge (\tr'=\tr) $} \\
     1 & \mbox{if $(\tr=1) \wedge (\tr'=\tr)$} \\
     0 & \mbox{otherwise;}
     \end{array}  \right.
     \]
    where $\lambda = 0.5$;
    
    \item for $(x,y),(x',y') \in \mathcal{R}$ and $a \in \Act$ if
     \[ \begin{array}{rcl}
     x'' & = & x - \Delta t d_{\mathit{ax}} \\
     y'' & = & y + \Delta t d_{\mathit{ay}}
     \end{array} \] 
     where $\Delta t = 1.0$ is the time step and $d_{a}  = (d_{\mathit{ax}}, d_{\mathit{ay}})$ is the direction of movement of the action $a$, e.g., $d_{\mathit{up}}=(0,1)$ and $d_{\mathit{left}}=(-1,0)$, then 
     \[
     \delta_E((x, y),a)(x', y') = \left\{ \begin{array}{cl}
     1 & \mbox{if $(x'',y'') \in \mathcal{R}$ and $(x',y')=(x'',y'')$} \\
     1 & \mbox{if $(x'',y'') \not\in \mathcal{R}$ and $(x',y')=(x,y)$} \\
     0 & \mbox{otherwise}
     \end{array}     \right.
     \]
    % \item 
    % The transition function of the environment corresponds to the vehicle moving in the direction specified by the agent for a fixed time step, unless the vehicle moves outside of $\mathcal{R}$ in which case it does not move. 
    %For $w \in S_E$ and $a \in \Act$, we let $\delta_E(w,a) = w'$ where $w’$ equals $w + d_{a} \Delta$ if $(w+ d_{a} \Delta t) \in S_E$ and equals $w$ otherwise,
%$d_{a}$ is the direction of movement of the action $a$, e.g., $d_{\mathit{up}}=(0,1)$ and $d_{\mathit{left}}=(-1,0)$ and $\Delta t = 1.0$ is the time step. 
\end{itemize}
In the reward structure, all action rewards are zero and the state reward function is such that for any $(s_A,(x,y)) \in S$:
\begin{align*}
r_S(s_A,(x,y)) &= \left\{ \begin{array}{cl}
 1000 & \mbox{ if $(x,y) \in \mathcal{R}_P$} \\
0 &  \mbox{otherwise}
\end{array} \right.
% r_S^2(s) &= \left\{ \begin{array}{cl}
% \!\!-1000 + \tr/20 & \!\! \mbox{if $t \in [0,1] \wedge h \in [-100,100]$} \\
% \!\!tr/20 & \!\! \mbox{otherwise.}
% \end{array} \right. 
\end{align*}
i.e., there is a positive reward if the parking spot is found.
%set the discount factor to be $\beta = 0.5$. 

\begin{table*}[t]
\setlength{\tabcolsep}{5pt}  
\centering
\scriptsize{
\begin{tabular}{|c|c||c|c||c|c||c|c|} \hline
Abstract & {\revise Intuitive}  & Abstract & {\revise Intuitive} & Abstract & {\revise Intuitive} &  Abstract & {\revise Intuitive} 
\\
grid {\revise cell} & actions & grid {\revise cell} & actions & grid {\revise cell} & actions & grid {\revise cell} & actions 
\\ \hline \hline	
$(1,1)$ & $\mathit{up}, \mathit{right}$ & $(1,2)$ &   $\mathit{up}, \mathit{right}$ & $(1,3)$ & $\mathit{up}, \mathit{right}$ & $(1,4)$ &  $\mathit{right}$ 
\\
$(2,1)$ & $\mathit{up}, \mathit{right}$ & $(2,2)$ &  $\mathit{up}, \mathit{right}$  & $(2,3)$ & $\mathit{up}, \mathit{right}$ & $(2,4)$ &  $\mathit{right}$ 
\\
$(3,1)$ & $\mathit{up}$  & $(3,2)$ &   $\mathit{up}$ &  $(3,3)$ & $\mathit{up}$ & $(3,4)$ &   $\mathit{park}$ 
\\
$(4,1)$ &  $\mathit{up}, \mathit{left}$ & $(4,2)$ & $\mathit{up}, \mathit{left}$ & $(4,3)$ &  $\mathit{up}, \mathit{left}$ & $(4,4)$ & $\mathit{left}$
\\ \hline
\end{tabular}}
\vspace*{-0.0cm}
\caption{{\revise Intuitive} actions of the agent for each percept (abstract grid cell) of the car parking example.}
\label{tab:advisory-parking}
\end{table*}

\iffalse
\begin{table*}[t]
% \renewcommand{\arraystretch}{1.5}
\setlength{\tabcolsep}{5pt}  
\centering
\scriptsize{
\begin{tabular}{|c|l|c|c|} \hline
Cell label & \multirow{2}{*}{Description} & Abstraction grid & \multirow{2}{*}{Suggested actions} \\
$(\per)$ & & (left $\to$ right, bottom $\to$ top) & 
 \\ \hline \hline	
1 & Left bottom to spot & $(1,1)$ & $\mathit{up}, \mathit{right}$
\\
2 & Left bottom to spot & $(2,1)$ & $\mathit{up}, \mathit{right}$ 
\\
3 & Bottom to spot & $(3,1)$ & $up$
\\
4 & Right bottom to spot & $(4,1)$ &  $\mathit{up}, \mathit{left}$
\\
5 & Left bottom to spot & $(1,2)$ &   $\mathit{up}, \mathit{right}$
\\
6 & Left bottom to spot & $(2,2)$ &  $\mathit{up}, \mathit{right}$
\\
7 & Bottom to spot & $(3,2)$ &   $\mathit{up}$
\\
8 & Right bottom to spot & $(4,2)$ & $\mathit{up}, \mathit{left}$
\\ 
9 & Left bottom to spot & $(1,3)$ & $\mathit{up}, \mathit{right}$
\\
10 & Left bottom to spot & $(2,3)$ & $\mathit{up}, \mathit{right}$ 
\\
11 & Bottom to spot &  $(3,3)$ & $\mathit{up}$
\\
12 & Right bottom to spot & $(4,3)$ &  $\mathit{up}, \mathit{left}$
\\
13 & Left to spot & $(1,4)$ &   $\mathit{right}$
\\
14 & Left to spot & $(2,4)$ &  $\mathit{right}$
\\
15 & At spot & $(3,4)$ &   $\mathit{parking}$
\\
16 & Right to spot & $(4,4)$ & $\mathit{left}$
\\ \hline
%
\end{tabular}}
\vspace*{0.2cm}
\caption{Suggested actions for each percept of car parking ($4\times 4$).}
\label{tab:advisory-parking}
\end{table*}
\fi

In this case of a $4{\times}4$ environment and no obstacles, for the region-based beliefs representation, \figref{fig:car_parking_region_plot} (left) presents the first four regions reached by the synthesised strategy for the initial state labelled by $\mathtt{x}$ in the initial region.
The belief at each step is the uniform distribution over the corresponding region and, as can be seen in the figure, the volume of the third region is smaller than that of the first and second regions. This reduction in volume is a result of the states reached from the states in the second region by performing action $\mathit{right}$ having different percepts, and therefore additional information about the environment state being obtained through the observation after the second transition.
%\gethin{larger probability density? The total probability is 1 so how is it larger?} \rui{yes. Since the area of the region becomes smaller and uniform closure holds, then the probability density has to be improved due to the total probability $1$. The reason why the region becomes smaller is because some states in the region cannot generate what the agent observes after taking an action. The density improves because the agent updates its belief as more information is obtained, meaning the agent is decreasing the uncertainties} \gethin{as I said the total probability remains 1 so the density is not larger}
%as the uniform distribution closure is kept. 
As can be seen in \figref{fig:car_parking_region_plot} (left), although the volume of the regions decreases, the actual state reached at each step (marked by $\mathtt{x}$), is consistently covered by the current region, thus ensuring the correctness of the region-based belief update.  
%\gethinM{how about this?} \ruiM{thanks, it looks very good}
%
%\gethin{what does diversity mean?} \rui{The diversity means that we need enough particles in the initial belief such that there exists at least one particle which can generate the same sequence of observations as the true state will generate given a sequence of actions; otherwise, the belief update will end suddenly.} \gethin{but we are using region-based not particle based beliefs?} \rui{yes, but region-based is for the belief representation. The current environment state cannot be a region but a point. For instance, the current position of the vehicle is a point not a region.} \gethin{so correctness of the belief update rather than diversity - since the current state is in the region?}
%
\figref{fig:car_parking_region_plot} (right) shows the lower and upper bound values
at each iteration, and the convergence demonstrates that the approximate upper bound for the region-based beliefs is tight if the belief has a unique region (see \lemaref{rb-upper-bound}).

%\rui{please check} \gethin{what is the true state? What if the true state was not covered by the current belief or can this not happen?} \rui{Whenever we synthesize a strategy for an instance, a true state (including the observable agent state and unobservable environment state) is needed. Since the agent doesn't know the true environment state and thus forms a belief, the agent then takes actions based on the beliefs and updates beliefs based on the observation generated by the true state. If the true state is not covered by the belief and gives an observation which never occurs based on the current belief, then the agent would know the current belief is incorrect. In our case, the initial true state is covered by the initial belief and there is no unknown transition, then we can guarantee that the true state is always covered by the current belief. This is why particle-based beliefs need a large number of particles for diversity to ensure that the particles in the current belief can always generate what the agent is observing.} \gethin{but no reader of the paper will know what true state means} \gethin{do we explain how strategies are synthesised using a true state?} \rui{yeah, we can just say the current state instead of "true" state}

\begin{figure}[t]
\centering
%\hspace{-1.0cm}
\raisebox{0.12\height}{
\begin{subfigure}{0.28\textwidth}
\includegraphics[width=\textwidth]{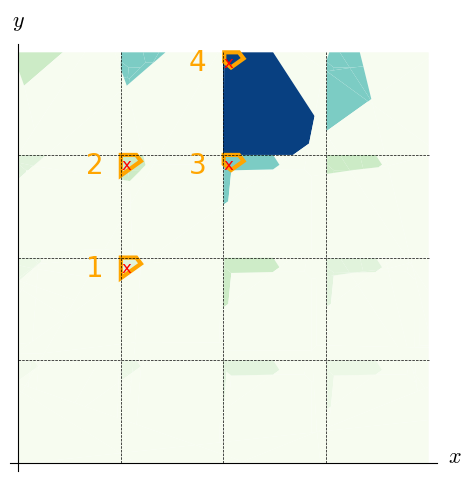}
\end{subfigure}
}
\hfil
\raisebox{0.04\height}{
\begin{subfigure}{0.1\textwidth}
\includegraphics[height=3.1\textwidth]{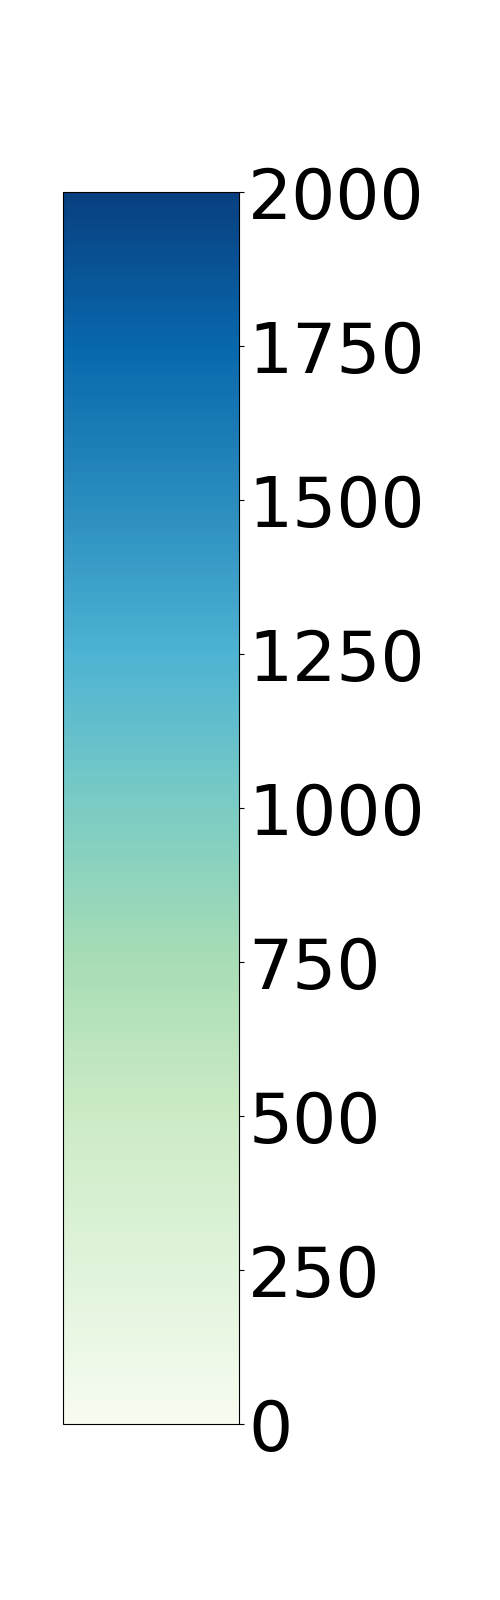}
\end{subfigure}
}
\hfil
\begin{subfigure}{0.5\textwidth}
\input{figures/parking/bounds_region.tex}
\end{subfigure}
\vspace*{-0.2cm}
\caption{Region-based paths and values for car parking (no obstacles).}
\label{fig:car_parking_region_plot}
\end{figure}

\begin{figure}[t]
\vspace*{-0.4cm}
\centering
\begin{subfigure}{0.25\textwidth}
\raisebox{0.3\height}{\scalebox{.6}{\input{figures/parking/parking-obstacle-4x4.tex}}}
\end{subfigure}
\hfil
\begin{subfigure}{0.3\textwidth}
\scalebox{.6}{\input{figures/parking/parking-obstacle-8x8.tex}}
\end{subfigure}
\caption{Car parking with obstacles.}
\label{fig:car_parking_obstacle}
\end{figure}

To extend this example to the case when there is an obstacle below the spot, i.e.,  an obstacle region is $\mathcal{R}_O = \{(x, y) \in \mathbb{R}^2 \mid 2 \leq x , y \leq 3\}$ see \figref{fig:car_parking_obstacle} (left), then the state reward function changes such that for any $(s_A,(x,y)) \in S$:
\begin{align*}
r_S(s_A,(x,y)) &= \left\{ \begin{array}{cl}
 1000 & \mbox{ if $(x,y) \in \mathcal{R}_P$} \\
 - 1000 &  \mbox{ if $(x,y)  \in \mathcal{R}_O$} \\
0 &  \mbox{otherwise}
\end{array} \right.
\end{align*}
i.e., there is a negative reward if the vehicle hits the obstacle.

\begin{figure}[t]
\centering
\scalebox{.5}{\includegraphics[width=\textwidth]{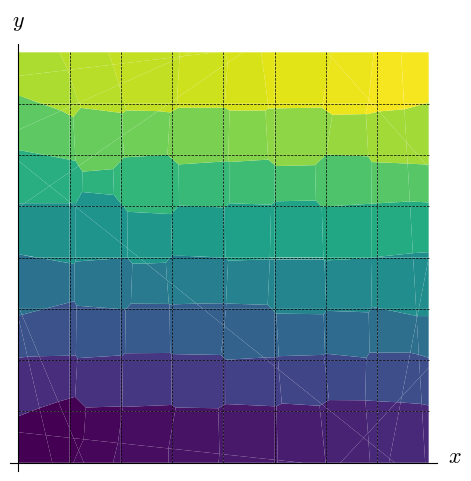}}
\put(-180,-3){\scriptsize $0$}
\put(-150,-3){\scriptsize $1$}
\put(-132,-3){\scriptsize $2$}
\put(-114,-3){\scriptsize $3$}
\put(-94,-3){\scriptsize $4$}
\put(-74,-3){\scriptsize $5$}
\put(-56,-3){\scriptsize $6$}
\put(-38,-3){\scriptsize $7$}
\put(-18,-3){\scriptsize $8$}
\put(-180,20){\scriptsize $1$}
\put(-180,40){\scriptsize $2$}
\put(-180,60){\scriptsize $3$}
\put(-180,80){\scriptsize $4$}
\put(-180,100){\scriptsize $5$}
\put(-180,118){\scriptsize $6$}
\put(-180,136){\scriptsize $7$}
\put(-180,154){\scriptsize $8$}
\vspace*{-0.2cm}
\caption{Perception FCP for car parking ($8\times 8$).}
\label{fig:car_parking_8x8_perception}
\end{figure}

% \ruiM{The illustration figures might be enlarged}

\startpara{$8 {\times} 8$ environment} We also consider a larger $8 {\times} 8$ environment $\mathcal{R}= \{(x, y) \in \mathbb{R}^2 \mid 0 \leq x, y \leq 8\}$ with 4 obstacles (\figref{fig:car_parking_obstacle}, right). In this model the parking spot is given by $\mathcal{R}_P = \{ (x,y) \in \mathbb{R}^2 \mid 6 \leq x  \leq 8 \wedge 7 \leq y \leq 8 \}$ and there are the following obstacle regions:
\[
\begin{array}{rcl}
\mathcal{R}_{O_1} &=& \{  (x,y) \in \mathbb{R}^2 \mid   4 \leq x \leq  5 \wedge 0 \leq y \leq 1 \} \\
\mathcal{R}_{O_2} &=& \{  (x,y) \in \mathbb{R}^2 \mid  7 \leq x \leq 8 \wedge 2 \leq y \leq  3 \} \\
\mathcal{R}_{O_3} &=&  \{  (x,y) \in \mathbb{R}^2 \mid 4 \leq x,y\leq  5 \} \\
\mathcal{R}_{O_4} &=&  \{  (x,y) \in \mathbb{R}^2 \mid  2 \leq x \leq 4 \wedge 7 \leq y \leq 8 \} \, .
\end{array}
\]
To extend the NS-POMP to this setting, the following changes to the components $S_A$, $S_E$, $\Delta_A$ and $\obs_A$ need to be made:
\begin{itemize}
	\item $S_A= \Loc \times \Per$ where 5 trust levels $\Loc = \{1,\dots,5\}$ and 64 abstract grid points $\Per = \{ 1, \dots, 64 \}$ (percepts) which are ordered in the same way as \tabref{tab:advisory-parking};

	\item $S_E = \mathcal{R}= \{(x, y) \in \mathbb{R}^2 \mid 0 \leq x, y \leq 8\}$;

	\item $\Delta_A(tr, \per) = \Act$ if $\per \in \{ 63 , 64 \}$ and $\Delta_A(tr, \per) = \{ \mathit{up}, \mathit{down}, \mathit{left}, \mathit{right} \} $ otherwise for all $tr \in \Loc$ and $\per \in \Per$;

	 \item $\obs_A(tr,(x, y))=\argmax (f(x,y ))$, where $f$ is implemented via a feed-forward NN with one ReLU hidden-layer with 15 neurons, takes the coordinate vector of the vehicle as input and then outputs one of the 64 abstract grid points.
\end{itemize}
In the reward structure, all action rewards are again zero and the state reward function is such that for any $(s_A,(x,y)) \in S$:
\begin{align*}
r_S(s_A,(x,y)) &= \left\{ \begin{array}{cl}
 1000 & \mbox{ if $(x, y) \in \mathcal{R}_P$} \\
 - 1000 & \mbox{ if $(x, y) \in \mathcal{R}_{O_i}$ and $1 \leq i \leq 4$} \\
0 &  \mbox{otherwise.}
\end{array} \right.
\end{align*}
%where  are the regions with obstacles, and set the discount factor to be $\beta = 0.7$.

%\gabriel{Entries in red had to be run on the laptop due to a library issue on Lovelace and thus are slower. Report them?} \gethin{the answer depends on whether they are much slower than the would be otherwise} \gabriel{Your guess is as good as mine. The only thing that can be said is that it probably would be quicker and thus, if people don't think they're too bad, they can be kept.} \rui{yeah, let's keep them}

\input{table_strat_stats.tex}

\begin{figure}[t]
\centering
\vspace{-0.5cm}
\begin{subfigure}{0.45\textwidth}
\includegraphics[width=\textwidth]{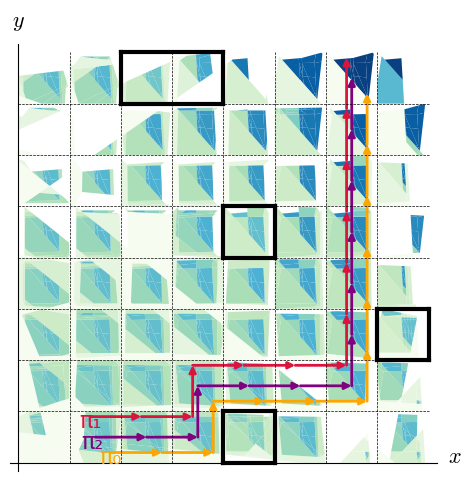}
\end{subfigure}
\hfil
\begin{subfigure}{0.48\textwidth}
\raisebox{-0.05\height}{\input{figures/parking/bounds_8X8.tex}}
\end{subfigure}
\vspace*{-0.2cm}
\caption{Paths and values for car parking ($8{\times}8$, partially reconstructed).}
\label{fig:car_parking_8x8_plot}
\end{figure}

\noindent
Table~\ref{tab:strat_stats} shows the total number of polyhedra that make up the alpha functions computed for each instance of the car parking case study, the lower and upper bound values (recall the accuracy for this case study is $10^{-3}$) and the time required for strategy synthesis, i.e., reading alpha functions, finding maximum actions and updating beliefs. The table also shows the compliance ratio with respect to the suggested actions, as well as the average trust values over 20 paths that were generated following the synthesised strategies. The following ratios  and trust values are both high for this case study as the suggested actions in \tabref{tab:advisory-parking} are close to the optimal strategies. 
%\gethin{updated - please check} \rui{looks fine, thanks}

\figref{fig:car_parking_8x8_perception} shows the perception FCP for the $8{\times} 8$ environment. For this extended model, \figref{fig:car_parking_8x8_plot} (left) presents the paths from the three particles in the initial belief for the synthesised strategy, as well as lower bound values for the regions of the environment. As the figure demonstrates, the vehicle is able to reach the parking spot while avoiding the obstacles. We should note that values are partially constructed by maximizing over a set of sampled $\alpha$-functions, as the full set of $\alpha$-functions is large (see Table~\ref{tab:strat_stats}), and therefore maximizing over all would require an even larger number of region intersections. \figref{fig:car_parking_8x8_plot} (right) presents how the lower and upper bound values for the initial belief change as the number of iterations of the NS-HSVI algorithm increases.

\subsection{VCAS Case Study}

%\subsection{VCAS}.

In this case study there are two commercial aircraft: an ownship aircraft equipped with an NN-controlled vertical collision avoidance system (VCAS) and an intruder aircraft. The avoidance system extends the classical VCAS~\cite{KDJ-MJK:19}, both adding trust to measure uncertainty and allowing for deviations from the advisories arising from the additional belief information.
Each second, 
% \gethin{why do we have a time step of 0.5 not 1?} 
the avoidance system  gives a vertical climb-acceleration  advisory $\ad$ to the pilot of the ownship to avoid near mid-air collisions (NMACs), which occur when the aircraft are separated by less than 100 ft vertically and 500 ft horizontally. Regarding the intruder, unlike the VCAS model considered~\cite{KDJ-MJK:19} we allow  a non-zero constant climb-rate for the intruder.

\begin{figure}[t]
\centering
\includegraphics[width=0.5\textwidth]{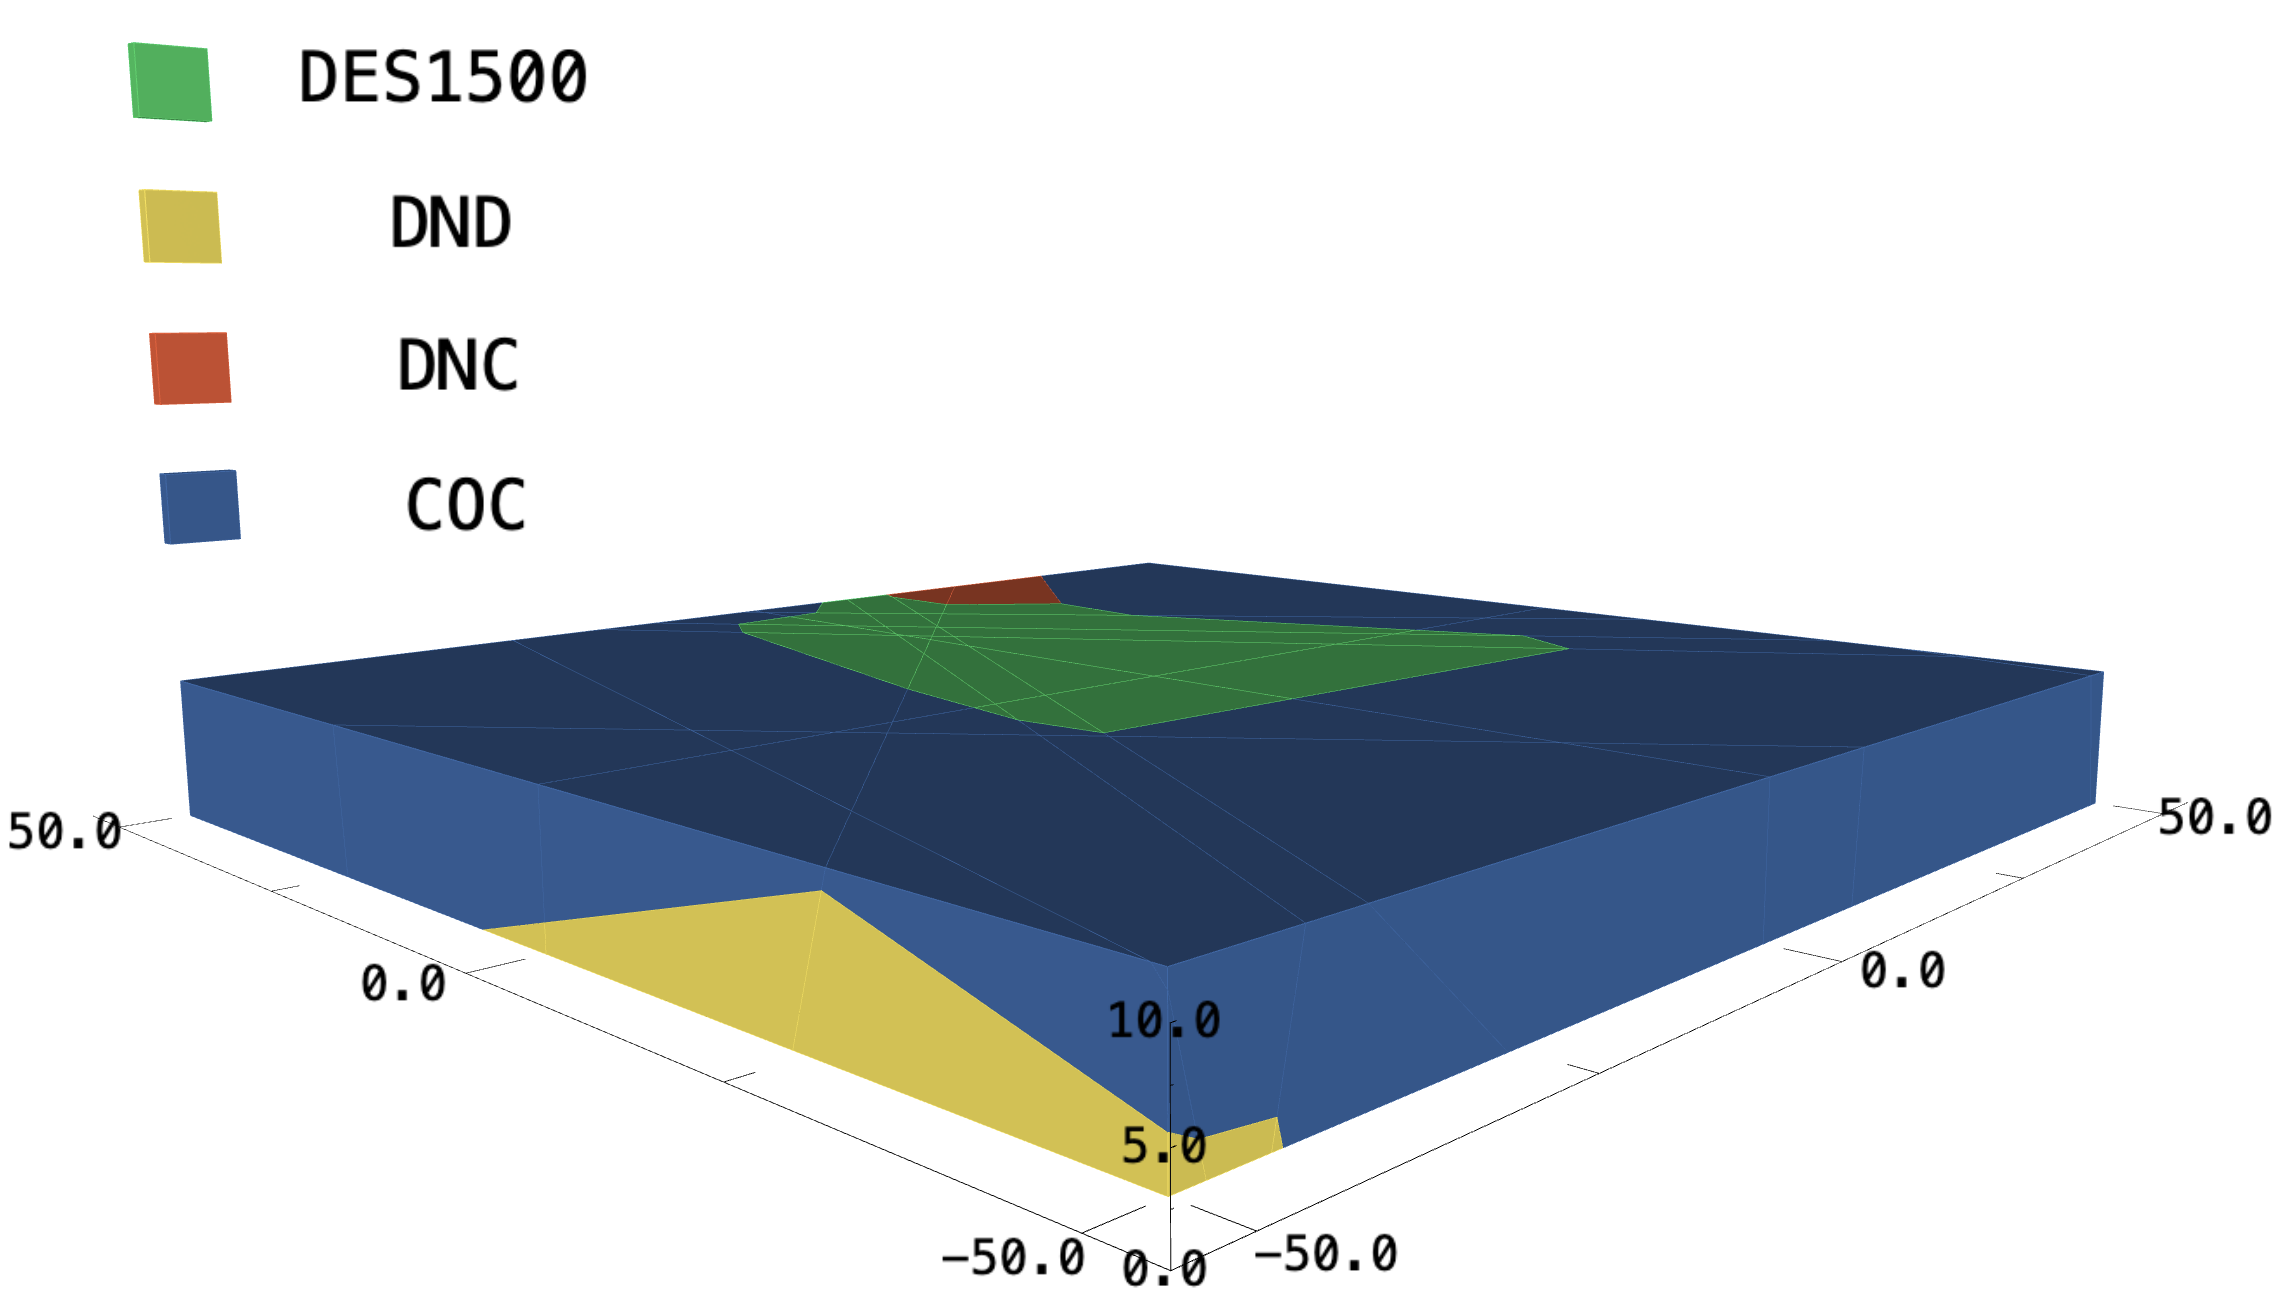}
\put(-175, 45){\scriptsize $t$}
\put(-30, 15){\scriptsize $h$}
\put(-160, 15){\scriptsize $\dot{h}_A$}
\caption{Slice of the FCP representation for the COC advisory ($h$ scaled 10:1).}
\label{FCP-COC}
\vspace*{-0.0cm}
\end{figure}
\input{figures/advisory_table}

%Below we give the formal definition of the $\agent$ and the environment $E$ of the VCAS case study. 

%Recall that input to VCAS is a tuple $(h, \dot{h}_A, t)$, where $h$ is the relative altitude of the two aircraft, $\dot{h}_A$ the climb rate of ownship, and $t$ the time  until the loss of horizontal separation between the aircraft and an environment state is such a tuple.
%Furthermore VCAS is implemented via nine feed-forward NNs $f_i:\mathbb{R}^3 \to \mathbb{R}^9$ for $1 \leq i \leq 9$, each of which outputs the scores of nine possible advisories, see \tabref{tab:advisory}. Each advisory provides a set of acceleration values and the ownship then either accelerates at one of these values or does not accelerate.

%The ownship which has four trust levels ($1$, $2$, $3$ and $4$), which represent the trust it has in the previous advisory. These levels increase if the current advisory is compliant with the executed action, and decrease with probability $\lambda(=0.5)$ otherwise. A local state of the agent is of the form $(\ad_\mathit{pre}, \tr)$ consisting of the previous advisory and the trust level and the percept of the agent is the current VCAS advisory.

\addtocounter{figure}{+1}

% \begin{figure*}[t]
% \centering
% \includegraphics[width=0.99\textwidth]{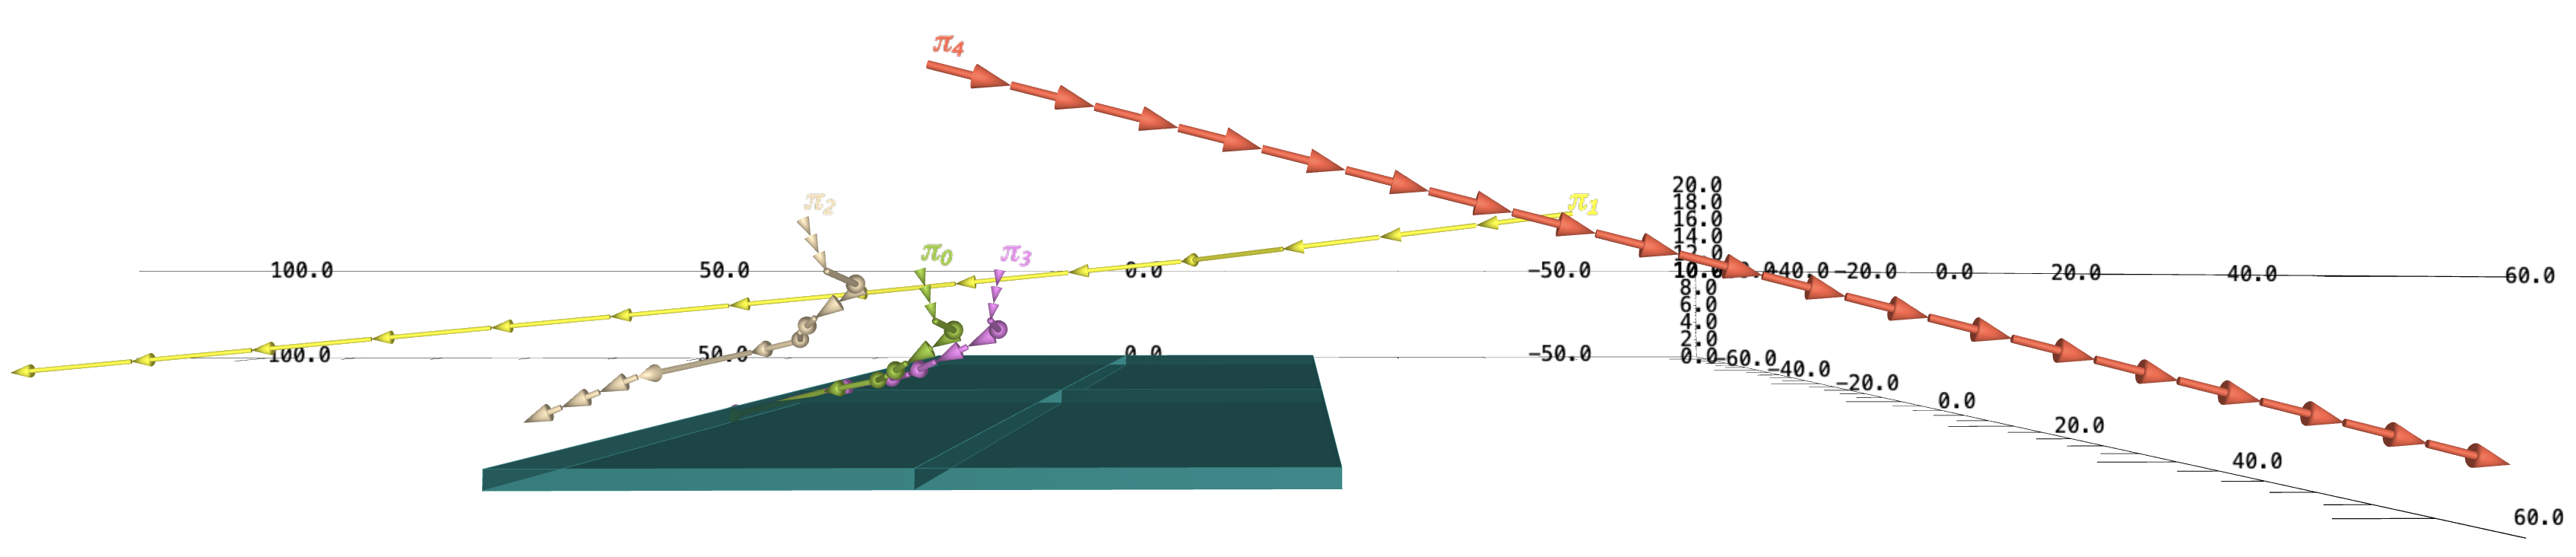}
% \put(-160, 75){\small $t$}
% \put(-280, -5){\small $h$}
% \put(-130, 18){\small $\dot{h}_A$}
% \caption{Additional paths constructed from a synthesised strategy showing both safe and unsafe scenarios ($h$ scaled 5:1).}
% \label{fig:supp:step_1}
% %\vspace*{-0.4cm}
% \end{figure*}

% \begin{figure*}
%     \begin{tikzpicture}
%     \node(a){\includegraphics[width=0.99\textwidth]{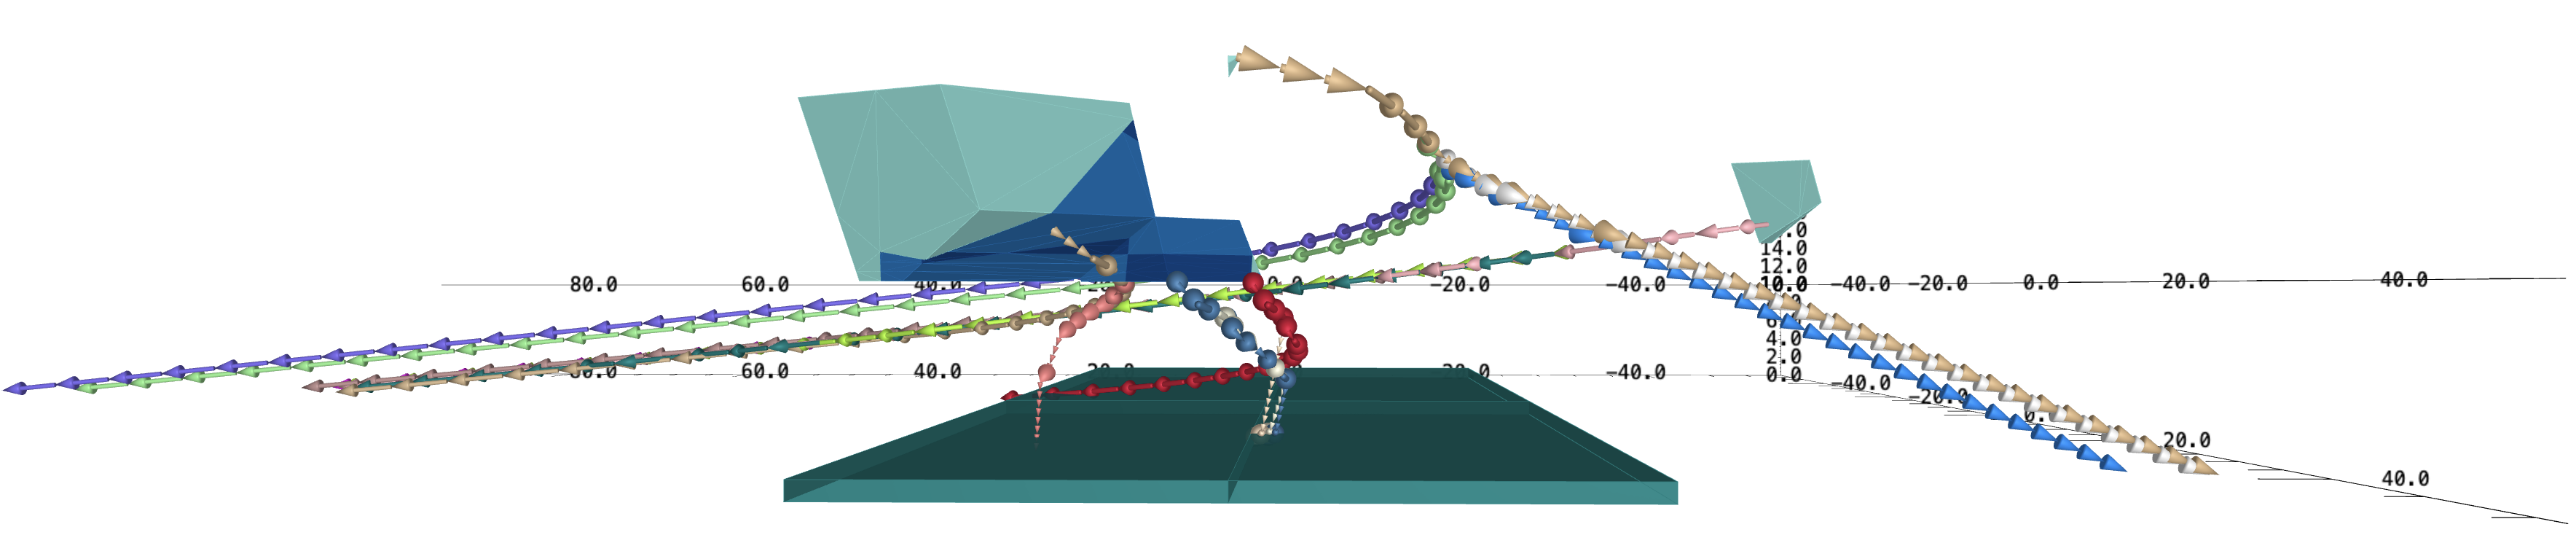}};
%     \node at (a.north east)
%     [
%     anchor=center,
%     xshift=-3.0cm,
%     yshift=0mm
%     ]
%     {
%         \includegraphics[height=0.8cm, width=0.4\textwidth]{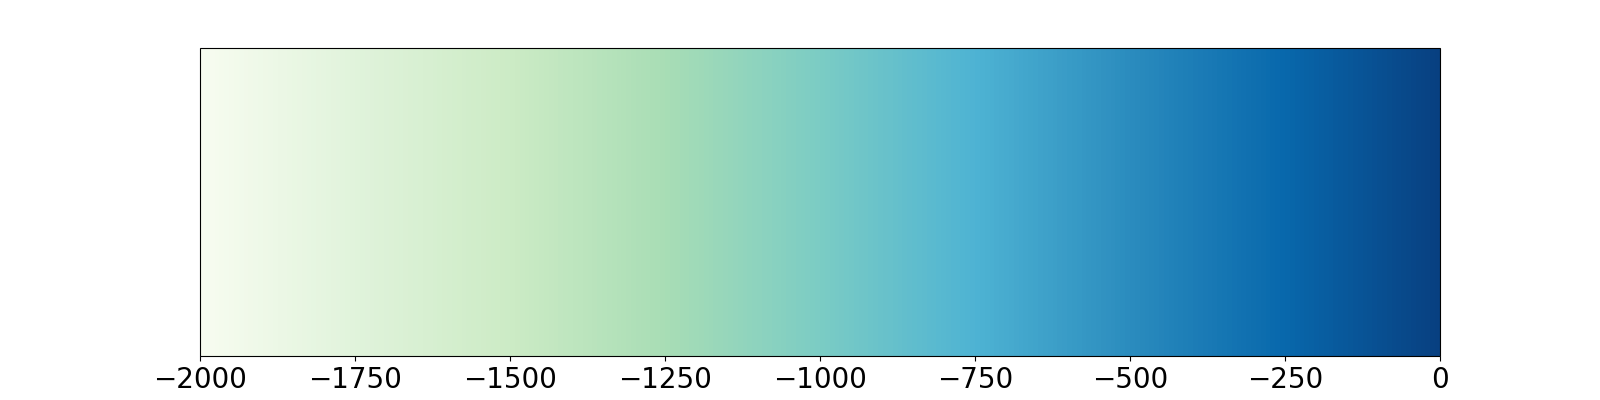}
%     };
%     \put(75, 15){\small $t$}
%     \put(0, -65){\small $h$}
%     \put(150, -18.5){\small $\dot{h}_A$}
%     \end{tikzpicture}
% \vspace*{0.05cm}
% \caption{Paths constructed from a synthesised strategy showing both safe and unsafe scenarios when the time step $\Delta t$ is changed to $0.5$ ($h$ scaled 5:1).}
% \label{fig:supp:regions}
% \end{figure*}

The input to VCAS is a tuple $(h, \dot{h}_A, t)$, where $h$ is the relative altitude of the two aircraft, $\dot{h}_A$ the climb rate of ownship, and $t$ the time  until the loss of horizontal separation between the aircraft. VCAS is implemented via nine feed-forward NNs %$f_i:\mathbb{R}^3 \to \mathbb{R}^9$ for $1 \leq i \leq 9$, 
each of which outputs the scores of nine possible advisories, see \tabref{tab:advisory}. Each advisory will provide a set of acceleration values and the ownship then either accelerates at one of these values or does not accelerate.
Each NN of VCAS has one ReLU hidden-layer with 16 neuros, and therefore the regions in its preimage are polytopes. If we had instead considered HorizontalCAS \cite{KDJ-MJK:19-2}, the nonlinear environment transition function twists polytopes into non-polytopes, and %\marta{but we say our method can cope with any regions, so this limitation is presumably due to the implementation} \rui{yes, our theoretical results apply to any regions, but due to the implementation challenge, we have to stick with polytopes} 
would destroy our finite representations. 

% \gethin{please check this is still correct}

% \gethin{this needs to go somehwere}
% We consider a more general constant climbrate $\dot{h}_{\text{int}} \in \mathbb{R}$ for the intruder $\agent_{\text{int}}$ than the work \cite{KDJ-MJK:19-2} in which $\agent_{\text{int}}$ is assumed to maintain level flight, i.e., $\dot{h}_{\text{int}} = 0$.

%\input{figures/advisory_table}

We model VCAS as an NS-POMDP in which the agent $\agent$ is the ownship.
The agent has four trust levels $\{1, \dots, 4\}$, which represent the trust it has in the previous advisory. These levels increase if the current advisory is compliant with the executed action, and decrease with probability $\lambda(=0.5)$ otherwise. A local state of the agent is of the form $(\ad_\mathit{pre}, \tr)$ consisting of the previous advisory and the trust level and the percept of the agent is the current VCAS advisory.
% The trust in the previous advisory and current advisory (percept) are stored in a state of the agent $s = (tr, ad)$. 
An environment state is a tuple $(h, \dot{h}_A, t)$ corresponding to the input of VCAS. Formally, we have:

\begin{itemize}
    \item $S_A= \Loc \times \Per$ where $\Loc = \{1,\dots,9\} \times \{1,\dots,4\}$ and $\Per = \{1,\dots,9\}$;
    
    \item $S_E = [-2000, 2000] \times [-50, 50] \times [0, 20]$;
    
    \item $\Act = \{0, \pm3.0, \pm7.33, \pm8.33, \pm9.33, \pm9.7, \pm10.7, \pm11.7 \}$;
    
     \item $\Delta_A(\loc, \per) = \Act$ for all $\loc \in \Loc$ and $\per \in \Per$;
     
    %  returns a set of non-zero acceleration actions \citep{MEA-EB-PK-AL:20} shown in Table \ref{tab:advisory} given a state of the agent, plus zero acceleration;
     
     \item $\obs_A((\ad_\mathit{pre}, \tr),s_E)=\argmax (f_{\ad_\mathit{pre}}(s_E))$, 
     where the boundary point is resolved by assigning the advisory with the smallest label in \tabref{tab:advisory}; 
    %  \gethin{what happens with ties?}
     
     \item for $s_A=((\ad_\mathit{pre},  \tr),\ad) \in S_A$, $(\ad', \tr') \in \Loc$ and $a \in \Act$, if $a$ is compliant with $\ad$ (see \tabref{tab:advisory}), then:
     \[
     \delta_A(s_A,a)((\tr',\ad')) = \left\{ \begin{array}{cl}
     1  & \mbox{if $(\tr\leq3) \wedge (\tr'=\tr+1) \wedge (\ad'=\ad)$} \\
     1 & \mbox{if $(\tr=4) \wedge (\tr'=\tr) \wedge (\ad'=\ad)$} \\
     0 & \mbox{otherwise}
     \end{array}  \right.
     \]
    if $a$ is not compliant with $\ad$, then:
     \[
     \delta_A(s_A,a)((\tr',\ad')) = \left\{ \begin{array}{cl}
     \lambda & \mbox{if $(\tr\geq 2) \wedge (\tr'=\tr-1) \wedge (\ad'=\ad)$} \\
     1-\lambda & \mbox{if $(\tr\geq 2) \wedge (\tr'=\tr) \wedge (\ad'=\ad)$} \\
     1 & \mbox{if $(\tr=1) \wedge (\tr'=\tr) \wedge (\ad'=\ad)$} \\
     0 & \mbox{otherwise;}
     \end{array}  \right.
     \]
     \item for $s=(h, \dot{h}_A, t),s'=(h', \dot{h}_A', t') \in S$ if
      \[ \begin{array}{rcl}
     h'' & = & h-\Delta t(\dot{h}_A-\dot{h}_{\textup{int}})-0.5\Delta t^2 \ddot{h}_A \\
     \dot{h}_A'' & = & \dot{h}_A+\ddot{h}_A\Delta t \\
     t'' & = & t-\Delta t
     \end{array} \]     
     then
     \[
     \delta_E(s,a)(s') = \left\{
     \begin{array}{cl}
     1 & \mbox{if $(h'', \dot{h}_A'', t'') \in S_E$ and $s'=(h'', \dot{h}_A'', t'')$} \\
     1 & \mbox{if $(h'', \dot{h}_A'', t'') \not\in S_E$ and $s'=s$} \\
     0 & \mbox{otherwise} \\
         \end{array} \right. \] 
     where $\Delta t = 1.0$ is the time step and the intruder is assumed to be a constant climb-rate $\dot{h}_{\text{int}} = 30$. 
     % \rui{please also rewrite the environment transition similar to the car parking example (does not move if going outside)} \gethin{what happens to $\dot{h}_A'$ in this case - is it still updated or does it also not change?} \rui{all variables don't change,} \gethin{should be fixed now} \rui{thanks}
\end{itemize}
In the reward structure we consider, all action rewards are zero and the state reward function is such that for any $s \in S$:
\begin{align*}
r_S(s) &= \left\{ \begin{array}{cl}
\!\!-1000 & \!\! \mbox{ if $t \in [0,1] \wedge h \in [-100,100]$} \\
\!\!0 & \!\! \mbox{otherwise}
\end{array} \right.
% r_S^2(s) &= \left\{ \begin{array}{cl}
% \!\!-1000 + \tr/20 & \!\! \mbox{if $t \in [0,1] \wedge h \in [-100,100]$} \\
% \!\!tr/20 & \!\! \mbox{otherwise.}
% \end{array} \right. 
\end{align*}
i.e., there is a negative reward if altitudes of the aircraft are within 100 ft at time 0 or 1, and set the discount factor to be $\beta = 0.5$.

To compute the perception FCP $\Phi_P$, i.e., the preimages of the NNs for this case study, we first trained these NNs. This involved computing an MDP table policy using local approximate value iteration, reformatting this into training data and training the NNs~\cite{KDJ-SS-JBJ-MJK:19}. To generate the preimages, we adapted the method of \cite{KM-FF:20}, computing exact preimages for the NNs of HorizontalCAS \cite{KDJ-MJK:19-2}. For example, the preimage for the COC (Clear of Conflict) advisory is shown in \figref{FCP-COC}, which shows VCAS next issuing the advisory DES1500 (Descend at least 1500 ft/min) for the environment states in the green region to avoid an NMAC given the small values of $h$ and $t$.

As for the car parking example, Table~\ref{tab:strat_stats} presents statistics for the $\alpha$-function representations, lower and upper bounds (recall the accuracy for this case study is $10^{-1}$) and time for strategy synthesis, as well as the following ratios and average trust values over 20 paths generated from the synthesised strategies. The $\alpha$-functions have a large number of regions as the perception FCP for each NN of the VCAS has many regions and there exist many intersections between the perception FCPs of the 9 NNs of this case study. 
%It should be noted that, due to the large number of actions and the limited number of paths, that measure does not reflect the inadequacy of the advisories as many actions could be optimal at any point. 
The following ratios and the average trust values are both low for this case study which is a result of the fact that many actions not suggested can ensure the safety and do not reflect inadequacies in the advisories.
